# Supplementary material for: Competition among Parallel Contests
Source: arXiv:2210.06866 source file (2022-10-27)
Supplement: Supplementary file 1 [file appendix.tex]

%\section{Missing Proofs in Section \ref{section:safetylevel}}
